# Supplementary material for: The mechanism of RNA base fraying: molecular dynamics simulations analyzed with core-set Markov state models
Source: arXiv:1811.12144 ancillary file (2019-03-07)
Supplement: Supplementary file 1 [file suppl.pdf]

# The mechanism of RNA base fraying: molecular dynamics simulations analyzed with core set Markov state models

## Supplementary Information

G. Pinamonti, F. Paul, F. Noè, A. Rodriguez, G. Bussi

## 1 Details of MD and MSM construction

Table SI 1 reports additional details regarding the MD simulations of the 4 RNA double helices simulated in this paper, as well as details about the trajectories of adenine di- and tri-nucleotide molecules, taken from Ref [1]. All trajectories were analyzed with the following protocol:

- MD data was stored with a stride, reported in Tab. SI 1, then G-vectors were computed with a cutoff of 0.24; backbone dihedrals and puckering angles were computed accordingly to the definitions given by `http://x3dna.org/highlights/torsion-angles-of-nucleic-acid-structures`.
- These coordinates were processed with TICA [2], using the lagtime reported in Tab SI 1, with kinetic map projection [3]; the number of TIC used in the rest of the analysis was selected with a cutoff in the kinetic variance of 0.9, and this number is reported in Tab. SI 1.
- The TWO-NN algorithm by Facco et al. [4] was used to estimate the intrinsic dimensionality of the TICA projected data, which is reported in Tab SI 1; PA$k$ [5] algorithm was used to compute the point-wise density in TICA space of each data point, $\rho$.
- DP clustering [6, 7] was used to cluster the data; the number of clusters resulting from the procedure is reported in Tab. SI 1.
- For each cluster, its core was defined as all points belonging to it, having $\rho > \rho_{\mathrm{MAX}} e^{-1}$, where $\rho_{\mathrm{MAX}}$ is the density of the cluster density peak; these were used for the successive core-based MSM construction.

| Molecule | N. traj. | Total length (μs) | Stride (ps) | TICA lagtime (ns) | TICA dimension | intrinsic dimension | k-means centers | UDP clusters |
|---|---|---|---|---|---|---|---|---|
| AA | 4 | 19.6 | 10 | 1.0 | 7 | 6 | 500 | 36 |
| AAA | 17 | 57.0 | 100 | 10.0 | 14 | 8 | 100 | 71 |
| ACGC | 32 | 53.5 | 100 | 5.0 | 16 | 9 | 500 | 197 |
| AGCC | 32 | 34.7 | 100 | 5.0 | 15 | 9 | 500 | 109 |
| UCGC | 32 | 47.6 | 100 | 5.0 | 13 | 9 | 500 | 99 |
| UGCG | 32 | 47.6 | 100 | 5.0 | 14 | 9 | 500 | 112 |

**Table SI 1:** Details of the MD simulations and of the MSMs. The systems consists in a) the adenine di- and tri-nucleotide (AA and AAA) already studied in Ref. [1] and b) the 4 duplexes simulated for the purpose of this study. Table shows details of the MD dataset (number of trajectories, and total simulated time), the stride used in the analysis, TICA lagtime and number of independent components considered, the intrinsic dimensionality as estimated by 2-nn algorithm.

# 2 States definition

Each microstate was classified using the following quantities:

1. average of RMSD with respect to native structure of a single terminal base, after optimal superposition of the structures with respect to the 3 G-C base pairs;
2. fraction of frames with stacking score $s > 0.05$, for each of the terminal bases with respect to the adiacent base;
3. Average of the $z$ component of the $G$ vector of a terminal base with respect to the adiacent base.

Then the classification is done as following:

- $C$: $\langle \text{RMSD} \rangle < 0.35$ nm for both bases;
- $O$: $\langle \text{RMSD} \rangle > 0.35$ nm, $s < 0.5$, $-0.04 < G_z < 0.04$, for both bases;
- $3P/5P$: RMSD of one base larger than 0.35, while the other fits the criteria for state $O$;
- $M$: none of the criteria above is fullfilled, and the 3' base has $G_z > 0.04$;
- $U$: all microstates not classified in the above categories.

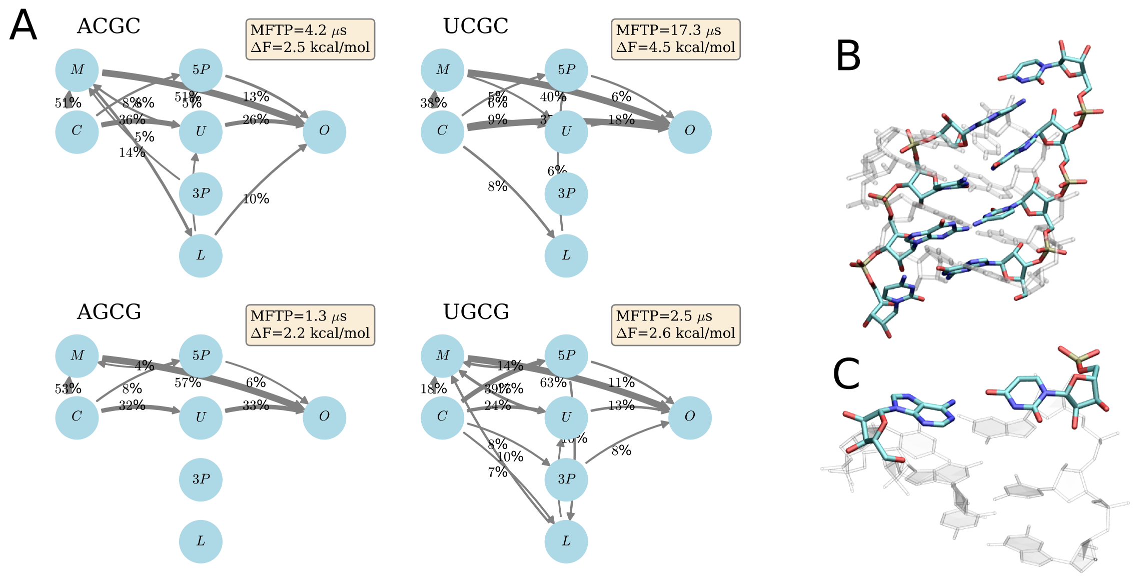


**Figure SI 1:** Results with the AMBER force field. Panel A: flux of fraying trajectories computed from the four MSM by means of TPT. Panel B: example of ladder-like structure, superimposed to a native A-form RNA helix (Sequence ACGC is shown as an example). Panel C: a typical misfolded structure for sequence ACGC. Bases A5' and U3' are highlighted as colored thick rods.

# 3 Supplementary results of kinetic analysis

Tables SI 2, SI 3, SI 4, and SI 5 report the stabilities of each state, as well as the average rates of transitions between them, computed as

$$\frac{1}{\tau}\sum_{j\in B}\left(\sum_{i\in A}\pi_i T_{ij}/\sum_{i\in A}\pi_i\right) \tag{1}$$

where $A$, $B$ are the initial and final state, $\pi_i$ is the equilibrium probability of microstate $i$, $T_{ij}$ is the transition probability from microstate $i$ to microstate $j$, $\tau$ is the lagtime used to construct the MSM.

## 3.1 Results of searches in the structural database

We searched all the nucleic-acids-containing structures deposited at `https://www.rcsb.org/` (retrieved on Oct 12, 2018) for fragments similar to those classified as misfolded in this study. In particular, for each construct we used as a query the most populated misfolded microstate. The unstacked nucleobase at the 5'-end was excluded from the query. Structures were searched for double-stranded motifs using Barnaba [8] with the command `barnaba DS_MOTIF --query query.pdb`

| $k$ (μs$^{-1}$) | $\Delta F$ (kcal/mol) | $C$ | $M$ | $U$ | $5P$ | $3P$ | $O$ |
|---|---|---|---|---|---|---|---|
| $C$ | −0.0 | | 0.2 | 0.6 | 1.0 | 0.3 | 0.0 |
| $M$ | 1.6 | 2.3 | | 1.6 | 0.0 | 28.7 | 1.7 |
| $U$ | 2.9 | 71.0 | 13.3 | | 67.5 | 17.6 | 5.8 |
| $5P$ | 2.4 | 57.7 | 0.0 | 33.7 | | 0.7 | 1.3 |
| $3P$ | 1.9 | 6.0 | 47.7 | 3.5 | 0.3 | | 2.2 |
| $O$ | 3.7 | 0.0 | 62.0 | 25.1 | 11.0 | 48.2 | |

**Table SI 2:** Rates and stabilities of the different states,from DESRES simulations for sequence ACGC

| $k$ (μs$^{-1}$) | $\Delta F$ (kcal/mol) | $C$ | $M$ | $U$ | $5P$ | $3P$ | $O$ |
|---|---|---|---|---|---|---|---|
| $C$ | −0.0 | | 0.1 | 0.5 | 2.2 | 0.2 | 0.0 |
| $M$ | 2.0 | 1.8 | | 1.5 | 0.0 | 48.1 | 5.8 |
| $U$ | 3.4 | 131.4 | 14.8 | | 122.9 | 0.0 | 14.8 |
| $5P$ | 2.0 | 59.6 | 0.0 | 11.8 | | 0.0 | 0.0 |
| $3P$ | 1.8 | 4.2 | 32.5 | 0.0 | 0.0 | | 4.0 |
| $O$ | 3.1 | 0.0 | 40.2 | 10.1 | 0.0 | 40.6 | |

**Table SI 3:** Rates and stabilities of the different states,from DESRES simulations for sequence AGCG

| $k$ (μs$^{-1}$) | $\Delta F$ (kcal/mol) | $C$ | $M$ | $U$ | $5P$ | $3P$ | $O$ |
|---|---|---|---|---|---|---|---|
| $C$ | −0.0 | | 0.0 | 0.1 | 2.2 | 0.0 | 0.0 |
| $M$ | 2.8 | 1.2 | | 1.2 | 1.2 | 11.2 | 2.5 |
| $U$ | 2.9 | 16.1 | 1.6 | | 42.8 | 1.6 | 0.0 |
| $5P$ | 1.6 | 29.6 | 0.2 | 4.2 | | 0.0 | 0.0 |
| $3P$ | 3.7 | 11.4 | 50.9 | 5.7 | 0.0 | | 11.3 |
| $O$ | 4.6 | 0.0 | 54.9 | 0.0 | 0.0 | 55.0 | |

**Table SI 4:** Rates and stabilities of the different states,from DESRES simulations for sequence UCGC

| $k$ (μs$^{-1}$) | $\Delta F$ (kcal/mol) | $C$ | $M$ | $U$ | $5P$ | $3P$ | $O$ |
|---|---|---|---|---|---|---|---|
| $C$ | −0.0 | | 0.1 | 0.2 | 10.5 | 0.1 | 0.0 |
| $M$ | 1.8 | 1.6 | | 0.4 | 1.9 | 13.8 | 8.4 |
| $U$ | 3.5 | 66.1 | 6.5 | | 88.7 | 57.6 | 7.3 |
| $5P$ | 0.4 | 19.7 | 0.2 | 0.5 | | 0.0 | 0.0 |
| $3P$ | 2.2 | 5.4 | 26.1 | 6.4 | 0.0 | | 14.4 |
| $O$ | 2.9 | 2.6 | 57.8 | 2.9 | 0.0 | 52.3 | |

**Table SI 5:** Rates and stabilities of the different states,from DESRES simulations for sequence UGCG

| Force field | Molecule | N. matches | eRMSD | PDB | Chain 1 | Residues 1 | Sequence 1 | Chain 2 | Residues 2 | Sequence 2 |
|---|---|---|---|---|---|---|---|---|---|---|
| | | | Best X-ray match | | | | | | | |
| DESRES | ACGC | 533 | 0.45 | 3JQ4 | A | 1449–1451 | CGC | A | 1571–1574 | GCGA |
| | AGCG | 254 | 0.48 | 4RGF | C | 27–29 | GGG | C | 38–41 | CCCU |
| | UCGC | 466 | 0.41 | 4R4V | A | 756–758 | AGC | A | 717–720 | GCUA |
| | UGCG | 221 | 0.33 | 3Q3Z | V | 40–42 | GCA | V | 66-69 | UGCA |
| AMBER | ACGC | 638 | 0.42 | 3JQ4 | A | 1449–1451 | CGC | A | 1571–1574 | GCGA |
| | AGCG | 295 | 0.39 | 3Q3Z | V | 40–42 | GCA | V | 66-69 | UGCA |
| | UCGC | 94 | 0.55 | 4R4P | A | 756–758 | AGC | A | 717–720 | GCUA |
| | UGCG | 349 | 0.44 | 3Q3Z | V | 40–42 | GCA | V | 66-69 | UGCA |

**Table SI 6:** Results of the search for fragments similar to the simulated structures classified as misfolded using both DESRES and AMBER force fields. The total number of matches is computed including all structures from the database. The best match is the fragment with the lowest eRMSD among those reported in X-ray diffraction experiments.

| $\Delta F$ (kcal/mol) | ACGC | AGCG | UCGC | UGCG |
|---|---|---|---|---|
| $M$ | −0.1 | −0.4 | 1.0 | 0.0 |
| $U$ | 1.2 | 0.2 | 0.8 | −0.2 |
| $5P$ | 1.8 | 0.3 | 1.5 | 0.3 |
| $3P$ | 2.3 | 2.1 | 2.7 | 2.1 |
| $O$ | 2.5 | 2.2 | 4.5 | 2.6 |

**Table SI 7:** Stabilities of different states from the MSM based on the AMBER simulations, with respect to the closed state $C$.

`--pdb database/*.pdb --l1 3 --l2 4 --threshold 0.7`. The 0.7 threshold for eRMSD [9] is expected to identify structures that have a virtually identical base-pair pattern [8]. The search is performed without constraining the sequence, so that the matching sequence might differ from the query one. The total number of matches and best match are reported in Table SI 6.

## 3.2 Supplementary results of AMBER simulations analysis

Tab SI 7 reports the stabilities of the different states computed from the MSM built on the AMBER simulations.

# References

[1] G. Pinamonti, J. Zhao, D. E. Condon, F. Paul, F. Noé, D. H. Turner, and G. Bussi, "Predicting the kinetics of RNA oligonucleotides using Markov state models," *J. Chem. Theory Comput.*, vol. 13, no. 2, pp. 926–934, 2017.

[2] G. Pérez-Hernández, F. Paul, T. Giorgino, G. De Fabritiis, and F. Noé, "Identification of slow molecular order parameters for Markov model construction," *J. Chem. Phys.*, vol. 139, no. 1, p. 015102, 2013.

[3] F. Noé and C. Clementi, "Kinetic distance and kinetic maps from molecular dynamics simulation," *J. Chem. Theory Comput.*, vol. 11, no. 10, pp. 5002–5011, 2015.

[4] E. Facco, M. d'Errico, A. Rodriguez, and A. Laio, "Estimating the intrinsic dimension of datasets by a minimal neighborhood information," *Sci. Rep.*, vol. 7, no. 1, p. 12140, 2017.

[5] A. Rodriguez, M. d'Errico, E. Facco, and A. Laio, "Computing the free energy without collective variables," *J. Chem. Theory Comput.*, vol. 14, no. 3, pp. 1206–1215, 2018.

[6] A. Rodriguez and A. Laio, "Clustering by fast search and find of density peaks," *Science*, vol. 344, no. 6191, pp. 1492–1496, 2014.

[7] M. d'Errico, E. Facco, A. Laio, and A. Rodriguez, "Automatic topography of high-dimensional data sets by non-parametric Density Peak clustering," *arXiv:1802.10549*, 2018.

[8] S. Bottaro, G. Bussi, G. Pinamonti, S. Reisser, W. Boomsma, and K. Lindorff-Larsen, "Barnaba: software for analysis of nucleic acid structures and trajectories," *RNA*, vol. 25, no. 2, pp. 219–231, 2019.

[9] S. Bottaro, F. Di Palma, and G. Bussi, "The role of nucleobase interactions in RNA structure and dynamics," *Nucleic Acids Res.*, vol. 42, no. 21, p. 13306, 2014.
